# Supplementary material for: Colloid-oil-water-interface interactions in the presence of multiple salts: charge regulation and dynamics
Source: arXiv:1703.08892 ancillary file (2017-06-07)
Supplement: Supplementary file 1 [file supplementary.pdf]

# Supplemental Information: Colloid-liquid-liquid-interface interactions in the presence of multiple salts: charge regulation and dynamics

J. C. Everts,[1] S. Samin,[1] N. A. Elbers,[2] J. E. S. van der Hoeven,[2] A. van Blaaderen,[2] and R. van Roij[1]

[1]*Institute for Theoretical Physics, Center for Extreme Matter and Emergent Phenomena, Utrecht University, Princetonplein 5, 3584 CC Utrecht, The Netherlands**

[2]*Soft Condensed Matter, Debye Institute for Nanomaterials Science, Princetonplein 5, 3584 CC, Utrecht, The Netherlands*

(Dated: March 27, 2017)

PACS numbers: 82.70.Kj, 68.05.Gh

## I. SALT EFFECTS OF CHARGED POLY(METHYLMETHACRYLATE) (PMMA) PARTICLES NEAR AN OIL-WATER INTERFACE

In this section we show some additional microscope images of charged PMMA particles near a water-cyclohexylbromide (CHB) interface and the influence of adding the salt tetrabutylammoniumbromide to either the water phase or oil phase. Finally, we show that the effects discussed in the main text for system 1 still hold under density-matching conditions.

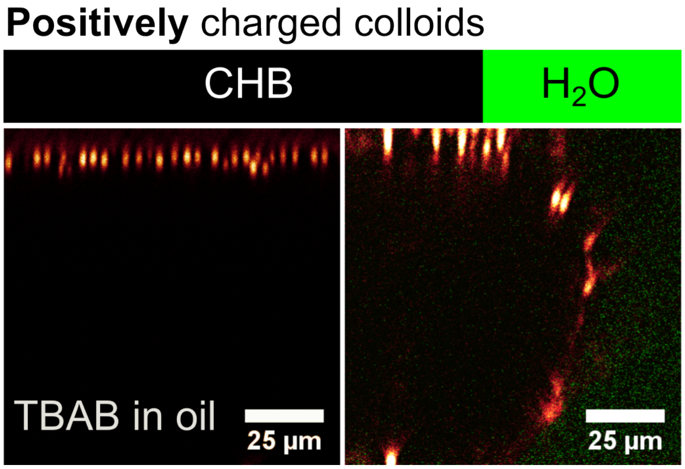


Figure S1. Confocal images of positively charged PMMA colloids in CHB in the bulk (left) and at the oil-water interface (right). Addition of 300 $\mu$M TBAB to the oil phase resulted in particle detachment (Figure 1, main text), but colloids were found to have reattached at the interface after 1 week of storage in a rotating stage as can be seen in the right image.

* jeffrey.everts@gmail.com

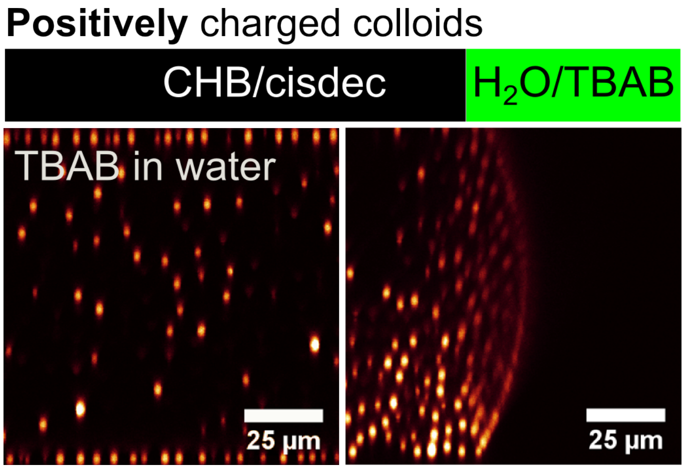


Figure S2. Positively charged PMMA colloids, dispersed in a mixture of CHB/27.2 wt% cisdecalin, were drawn from the oil to the oil-water interface when adding 50 mM TBAB to the water phase.

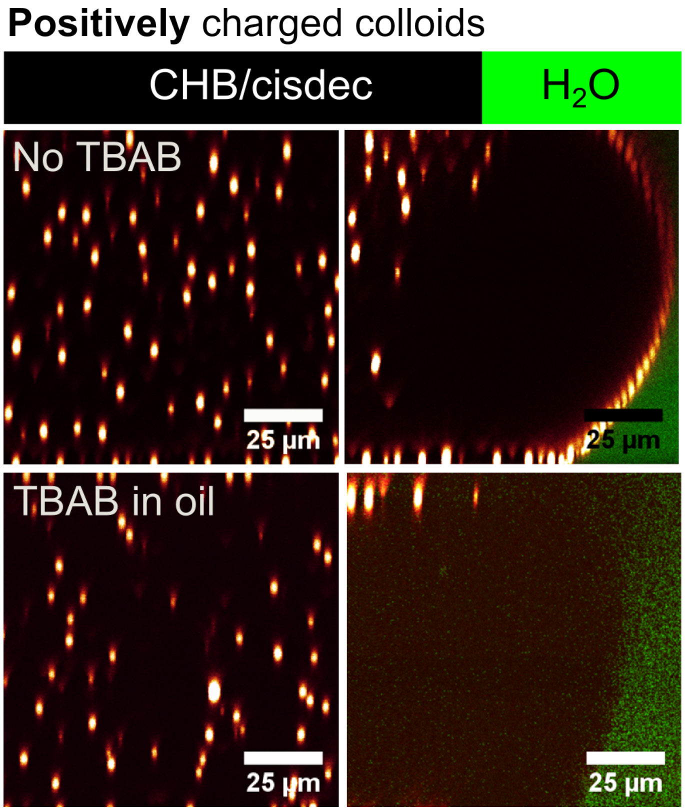


Figure S3. Confocal images of positively charged PMMA colloids dispersed in a mixture of CHB/27.2 wt% cisdecalin before (top) and after (bottom) the addition of 300 $\mu$M TBAB to the oil phase. Upon the addition of salt to the system the PMMA colloids detached from the oil-water phase.

.
